# Supplementary material for: Quantum Interference of Identical Photons from Remote GaAs Quantum Dots
Source: arXiv:2106.03871 source file (2023-02-14)
Supplement: Supplementary file 1 [file supplement_info.pdf]

# Supplementary Information: Quantum Interference of Identical Photons from Remote GaAs Quantum Dots

Liang Zhai,[1] Giang N. Nguyen,[1] Clemens Spinnler,[1] Julian Ritzmann,[2] Matthias C. Löbl,[1] Andreas D. Wieck,[2] Arne Ludwig,[2] Alisa Javadi,[1] and Richard J. Warburton[1]

[1] *Department of Physics, University of Basel, Klingelbergstrasse 82, CH-4056 Basel, Switzerland*
[2] *Lehrstuhl für Angewandte Festkörperphysik, Ruhr-Universität Bochum, DE-44780 Bochum, Germany*

## Supplementary Note 1. Hong-Ou-Mandel Interference from Single GaAs Quantum Dots

In the Hong-Ou-Mandel (HOM) as well as the associated Hanbury Brown-Twiss experiments, the photons created by a quantum dot (QD) pass through a 22 GHz-bandwidth grating-based filter (Supplementary Fig. 1). The grating (WasatchPhotonics, 1650 l/cm at 781 nm) has an efficiency of $\sim 80\%$. As the picosecond pulsed laser (duration 6 ps) is spectrally broad ($\sim 150$ GHz), the 22 GHz-bandwidth filter helps remove back-scattered laser light in the detection channel[1]. It is also essential for filtering out the weak phonon sideband (which constitutes 4% of the emission; the full width at half maximum is $\sim 0.6$ nm or equivalently 300 GHz; see Supplementary Fig. 2) and the even weaker radiative Auger emission[2] ($\sim 3$ THz away from the resonance fluorescence). The grating-based filter has little impact on the spectral (or temporal) profile of the zero-phonon line photons (Supplementary Fig. 1), since the grating's bandwidth is $\sim 40$ times larger than the QDs' linewidth. Therefore, the grating filter induces negligible spectral filtering effects to the zero-phonon line emission.

The one-QD HOM experiments are performed using a Mach-Zehnder interferometer[3,4] sketched in Supplementary Fig. 3. The photons are split equally into two arms and overlap on a fibre-based 50:50 beamsplitter. The photons travelling through the long arm experience a delay $\mathcal{D}$ compared to the shorter arm. In our experiments, we finely adjust the movable delay so that the delayed photon matches temporally with the $\mathcal{N}$th successively emitted photon. For $\mathcal{N} = 1$, $\mathcal{D} = 13$ ns; for $\mathcal{N} = 77$, $\mathcal{D} = 1.01$ $\mu$s. To characterise the HOM visibility, photons in the two arms are prepared in the same (HOM $\parallel$) and in the opposite polarisation (HOM $\perp$). A fibre-based polarisation controller is used to maximise (minimise) the classical interference visibility of the two arms when they are co-polarised (cross-polarised). For $\mathcal{D} = 13$ ns, the classical interference visibility is 99.8% (co-polarised) and 1.0% (cross-polarised); for $\mathcal{D} = 1.01$ $\mu$s, the contrast is slightly reduced to 99.5%/1.5% by the 200-metre fibre. At the two output ports of the beamsplitter, the QD photons are recorded using two superconducting nanowire single-photon detectors (SNSPDs) and a photon-counting hardware (Time Tagger Ultra, Swabian Instruments).

The raw HOM data of QD1 and QD2 are presented in Supplementary Fig. 4 and Supplementary Fig. 5 for the 13 ns and 1.01 $\mu$s delay, respectively. For the 13 ns case (1.01 $\mu$s case), the intensity of the $1^{\text{st}}$ ($77^{\text{th}}$) side peaks is 75% with respect to the other side peaks. The is a result of the route probability in the Mach-Zehnder interferometer. Since the QD creates single photons, a photon arriving at the first 50:50 beamsplitter is either transmitted, making its way to the short path of the interferometer, or reflected to the long arm. Thus, for two photons to be counted coincidentally, there exist four route probabilities: (i) both the two photons enter the long path, (ii) both enter the short path, (iii) the early photon enters the short path and the late photon the long path, and (iv) the early photon enters the long path and the late photon the short path. Depending on the route, the Mach-Zehnder interferometer induces different temporal delays to the photon pairs. To be specific, for (i) and (ii), the interferometer induces no delay; for (iii), a delay of $\mathcal{D} = \mathcal{N}T_{\text{period}}$ is induced; for (iv), a delay of $(-\mathcal{D})$ is induced. For all the side peaks except for the $\mathcal{N}^{\text{th}}$ ones, all four probabilities contribute to the coincidence events. For the $\mathcal{N}^{\text{th}}$ side peaks ($\tau = \pm\, \mathcal{N}T_{\text{period}}$), three out of four probabilities are accounted for. The missing probability is due to the fact that the two photons cannot be emitted at the same time by a single-photon emitter. (If two photons arrive at the first beamsplitter at the same time, then adding or subtracting a delay $\mathcal{D}$ leads to coincidence counts at the $\mathcal{N}^{\text{th}}$ side peaks. But this is not possible.) This is the reason why the $1^{\text{st}}$ and the $77^{\text{th}}$ side peaks are only 75% intensity in Supplementary Fig. 4 and Supplementary Fig. 5.

The raw visibility of the HOM interference is calculated as the ratio of the normalised area underneath the central peaks for the co- and cross-polarised measurements, $\mathcal{V}_{\text{raw}} = 1 - \frac{A_{\parallel}}{A_{\perp}}$. For the area calculation, we take into account the whole pulse period, i.e. $T_{\text{bin}} = 13$ ns. This binning size is $\sim 50$ times larger than the QD's lifetime – no temporal post-selection is introduced.

Experimental imperfections as well as the finite value of $g^{(2)}(0)$ influence the measured HOM visibility $\mathcal{V}_{\text{raw}}$. The second-order correlation functions $g^{(2)}(0)$ of the two QDs are measured in Hanbury Brown-Twiss measurements[4,5]. For this, we block one arm of the Mach-Zehnder interferometer and send the QD photons through the symmetric beamsplitter. The results are shown in Supplementary Fig. 6. We extract the $g^{(2)}(0)$ from the normalised central peak intensity: $g^{(2)}(0) = (1.3 \pm 0.2)\%$ for QD1 and $g^{(2)}(0) = (1.0 \pm 0.1)\%$ for QD2. Following Eq. (2) in the Methods

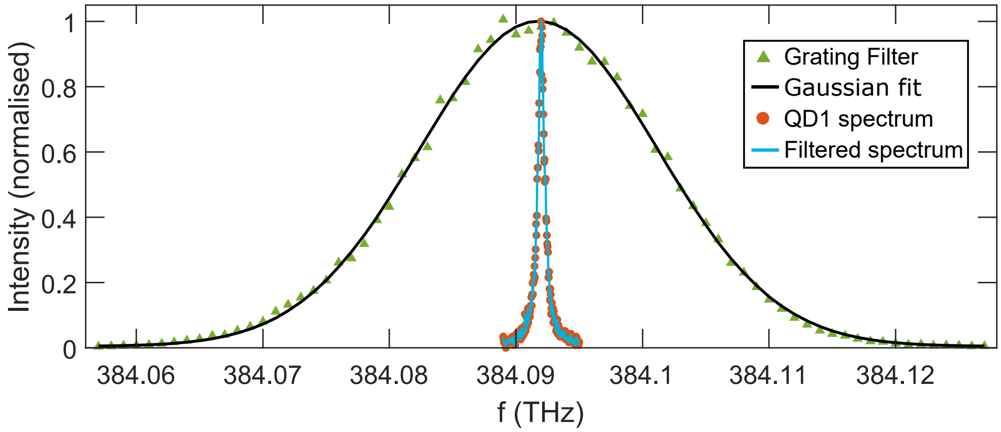


Supplementary Fig. 1. **The grating filter and its effect on quantum dot linewidths.** Green triangles represent the frequency dependence of the grating setup. The grating is aligned such that the first-order diffraction is focused by an achromatic lens ($f = 50$ mm) into a single-mode optical fibre. The grating filter has a bandwidth of 22.1 GHz (full-width-at-half-maximum) and follows a Gaussian profile (black curve). It is centred around the QDs' zero-phonon line. The red circles show the measured QD1 resonance fluorescence without passing through the grating, while the blue solid curve represents the expected spectrum with the grating filter in place. The perfect overlap between the red circles and the blue line confirms that the grating filter has little impact on the QD lineshape.

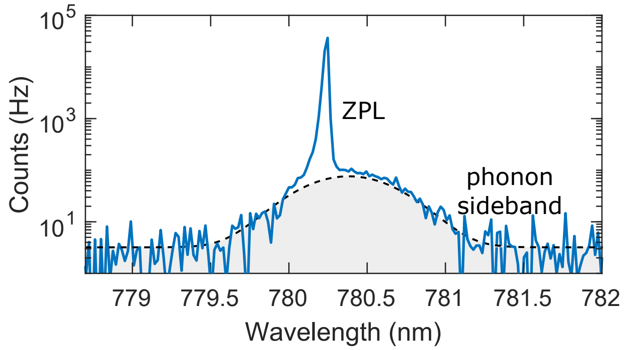


Supplementary Fig. 2. **The zero-phonon line and the phonon sideband emission in resonance fluorescence.** The resonance fluorescence is spectrally resolved with a spectrometer on tuning a CW laser into resonance with the QD2 $X^-$. The black dashed curve represents a guide to the eye for the phonon sideband emission. The phonon sideband is about 300 GHz in width (FWHM), constituting only 4% of the total emission. The zero-phonon line (ZPL) contributes 96% to the resonance fluorescence spectrum.

section, we correct $\mathcal{V}_{\text{raw}}$ with the finite $g^{(2)}(0)$ value and obtain the true one-QD HOM visibility. For QD1, we arrive at $\mathcal{V}^{13\text{ns}} = (97.8 \pm 1.8)\%$ and $\mathcal{V}^{1\mu\text{s}} = (99.0^{+1.0}_{-1.8})\%$; for QD2, we have $\mathcal{V}^{13\text{ns}} = (98.2 \pm 1.3)\%$, $\mathcal{V}^{1\mu\text{s}} = (98.7^{+1.3}_{-2.0})\%$.

### Supplementary Note 2. Hong-Ou-Mandel Interference from Two Remote Quantum Dots

To test the indistinguishability of photons from remote GaAs QDs (two-QD HOM), we employ the setup in Supplementary Fig. 7. We synchronise the excitation of the two QDs so that the two photons from the distant QDs arrive simultaneously at a 50:50 fibre-based beamsplitter. The synchronisation is achieved with a precision of $\pm 4$ ps by both a movable delay line and an exchangeable fibre delay in the excitation paths. Back-reflected laser light is rejected using a dark-field microscope[7] on each cryostat. Single photons from the two QDs pass through a half-wave plate (HWP) and a polarising beamsplitter (PBS) in the two separate collection paths – where the photon fluxes from both QDs are matched. 22 GHz-bandwidth grating filters are inserted before the SNSPDs to improve the laser suppression and to remove the phonon sideband and radiative Auger emissions[2].

The HOM interference of remote-QD photons is shown in Supplementary Fig. 8. The raw HOM visibilities for photons generated between QD1 and QD2 (90.9%) and between QD1 and QD3 (90.6%) are very similar. In analogy to the one-QD HOM, experimental imperfections and the finite $g^{(2)}(0)$ are accounted for in order to determine the

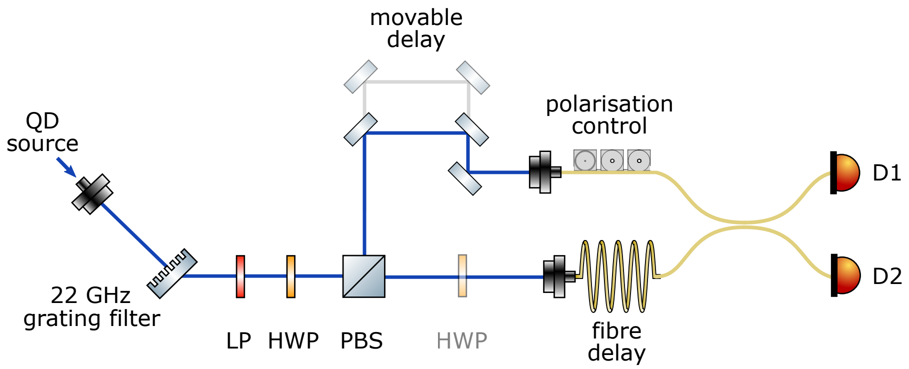


Supplementary Fig. 3. **Interferometry setup for one-quantum-dot Hong-Ou-Mandel experiments.** The QD photons are passed through a 22 GHz-bandwidth grating filter and sent to an unbalanced Mach-Zehnder interferometer. The interferometer has a "long" arm with an exchangeable fibre delay, and a "short" arm on a manual delay line. A linear polariser (LP), a half-wave plate (HWP), and a polarising beamsplitter (PBS) are used to balance the power in the two arms. The inserted fibre is 2-metre long for 13 ns ($\mathcal{N} = 1$) delay and 200-metre long for 1.01 $\mu$s delay ($\mathcal{N} = 77$). The photons travelling through the two arms impinge on a fibre-based 50:50 beamsplitter. The temporal overlap of the two arms is carefully adjusted by the movable delay line. A HWP in the long arm is employed on changing from the co-polarised configuration to the cross-polarised configuration. The photons in the two outputs are counted using two superconducting nanowire single-photon detectors ($D_1$ and $D_2$) and a streaming time-to-digital converter.

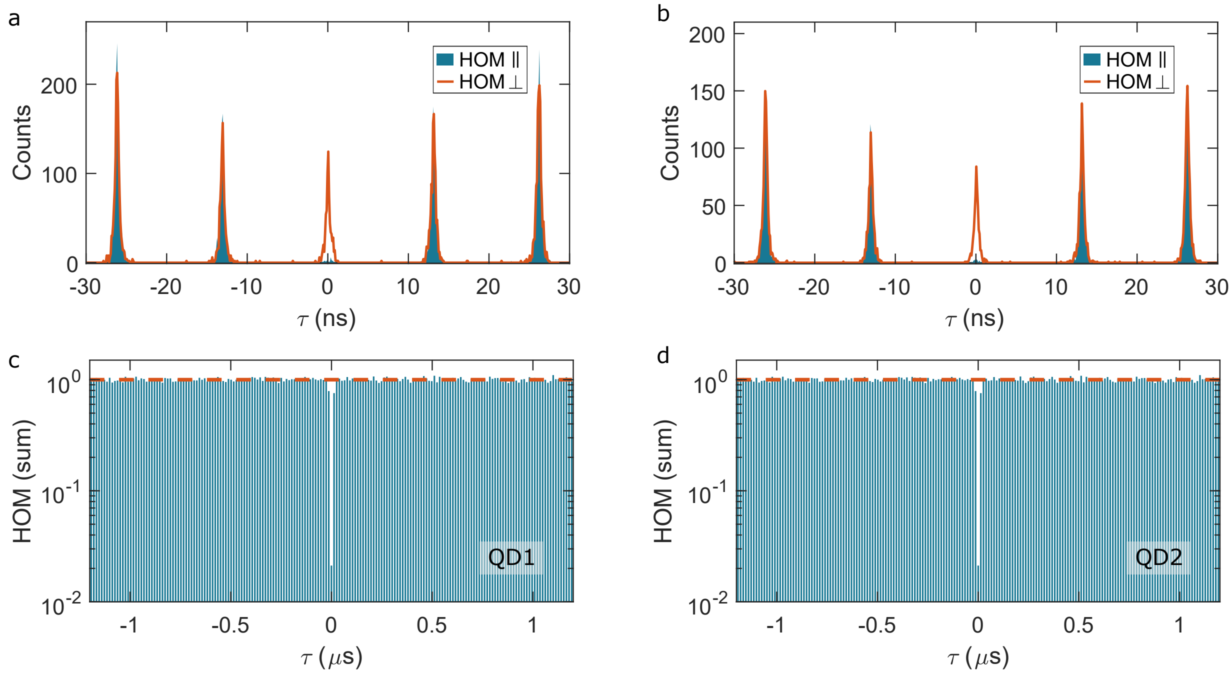


Supplementary Fig. 4. **Hong-Ou-Mandel interference between** 13 ns**-delayed photons from individual GaAs quantum dots. (a,b)** Time-resolved HOM interference in co-polarised (cyan) and cross-polarised (red) configurations for QD1 (a) and QD2 (b). The raw HOM visibility is extracted by calculating the ratio between the central peak areas in the two configurations. The area comprises the sum of all coincidence events in one pulse period around the zeroth peak, i.e. from $\tau = -6.5$ ns to $\tau = +6.5$ ns and is normalised by that of the side peaks. **(c,d)** The normalised HOM interference in co-polarised configuration for the two QDs. Each bar represents the sum of coincidence events around the peak at the corresponding $\tau$ using the full pulse period as the time binning window, $T_{\mathrm{bin}} = 13$ ns. The intensities of the bars are normalised at very long delay. The normalised HOM bars are flat showing an elimination of blinking. The intensity of the first bars ($i = \pm 1$) drops to 75% due to route probability, indicating that the quantum interference is measured between the consecutively emitted photons ($\mathcal{N} = 1$).

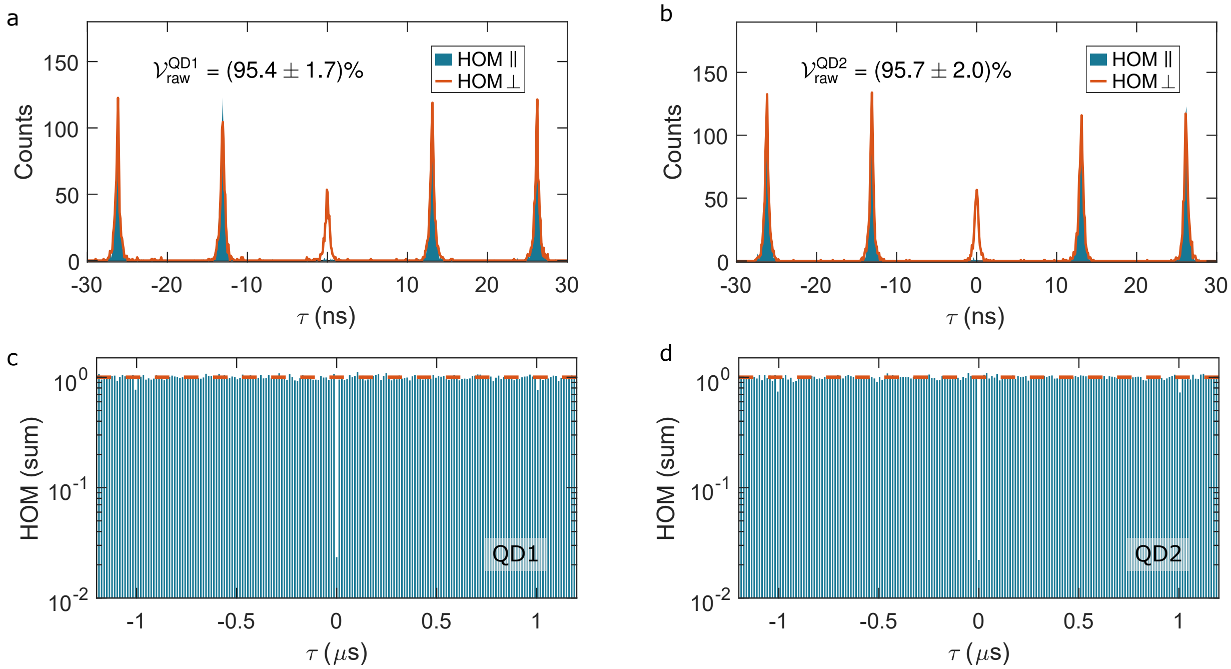


Supplementary Fig. 5. **Hong-Ou-Mandel interference between** 1.01 $\mu$s**-delayed photons from individual GaAs quantum dots.** **(a,b)** The time-resolved HOM interference in co-polarised (cyan) and cross-polarised (red) configurations for QD1 and QD2. **(c,d)** The normalised HOM interference in the co-polarised configuration for the two QDs. The time bin is $T_{\mathrm{bin}} = 13$ ns for every bar. The normalised HOM bars are flat out to a microsecond. The intensity of the 77$^{\mathrm{th}}$ bars ($i = \pm 77$) drops to 75% due to route probability, indicating that the quantum interference is measured between the photons emitted 77 pulse periods apart ($\mathcal{N} = 77$).

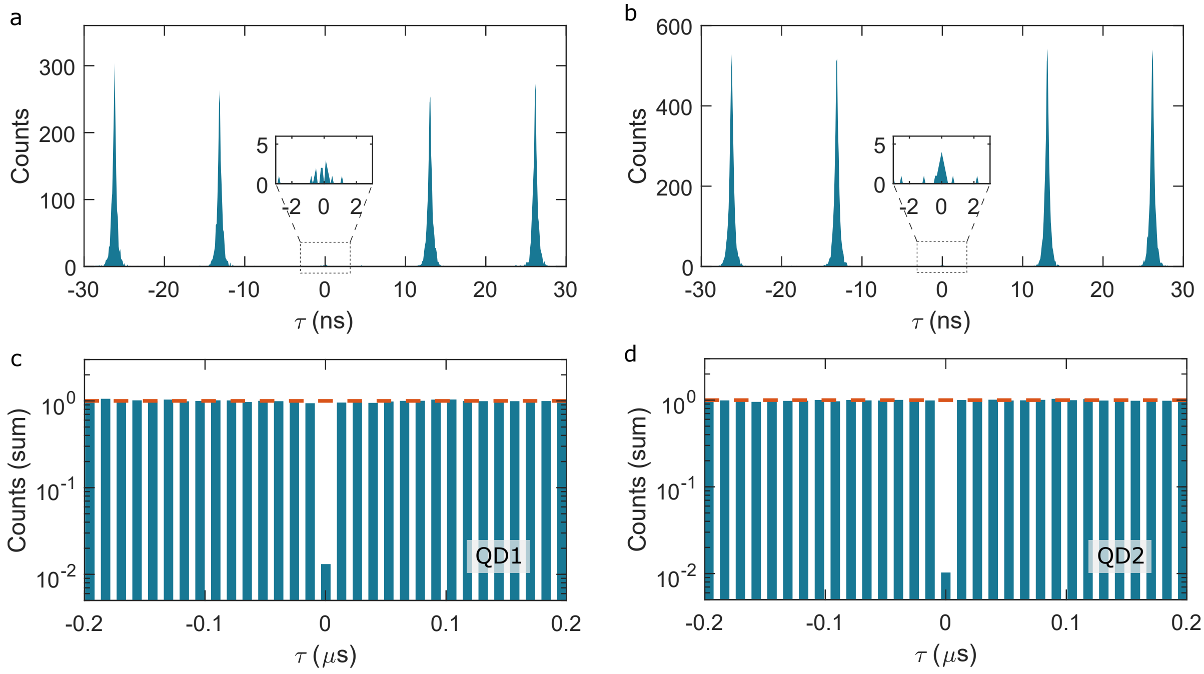


Supplementary Fig. 6. **Hanbury Brown-Twiss measurements on QD1 and QD2.** **(a,b)** Time-resolved auto-correlation of QD1 (a) and QD2 (b) under resonant pulsed excitation. The central peak in each plot is enlarged and displayed as an inset. The ratio between the central peak intensity and the average intensity of the side peaks defines $g^{(2)}(0)$. These ratios are more clearly visible in **(c,d)**, where coincidence counts in the time-resolved measurements are summed up peak by peak and normalised at long delays. The time bin is a whole pulse period ($T_{\mathrm{bin}} = 13$ ns). The central peak for both QDs reduces to $\sim 1\%$ indicating a high single-photon purity. The small but finite $g^{(2)}(0)$ comes likely from a re-excitation process[6].

true overlap $\mathcal{V}$ from the raw HOM visibility $\mathcal{V}_{\mathrm{raw}}$.

We outline the derivation of the relationship between $\mathcal{V}_{\mathrm{raw}}$ and $\mathcal{V}$. Considering two photons incident on a beamsplitter ($\tilde{BS}$) from the two input ports "$i$" and "$j$", the output after the beamsplitter in ports "$k$" and "$l$" can be calculated via:

$$|\mathrm{out}\rangle = \tilde{BS}\,|1_i, 1_j\rangle = t^2\,|1_l, 1_k\rangle - r^2\,|1_l, 1_k\rangle + i\sqrt{2}rt\Big(\,|2_l, 0_k\rangle + |0_l, 2_k\rangle\,\Big), \tag{1}$$

where $t^2 = T$ ($r^2 = R$) is the transmission (reflection) coefficient of the beamsplitter. The visibility of two-photon quantum interference for an ideal input $|1_i, 1_j\rangle$ is hence given by

$$\mathcal{V}_{\mathrm{Q}} = (t^2 - r^2)^2 = 1 - 4RT. \tag{2}$$

Here, we make use of the relation $T^2 + R^2 = 1$ and assume the two input photons are completely indistinguishable. When the two input photons are distinguishable, all quantum effects disappear and we arrive at the classical visibility:

$$\mathcal{V}_{\mathrm{C}} = |t^2|^2 + |r^2|^2 = 1 - 2RT. \tag{3}$$

The visibility in the case of quantum interference can be further expressed as:

$$\mathcal{V}_{\mathrm{Q}} = \mathcal{V}_{\mathrm{C}} - (1-\epsilon)^2\mathcal{V}(2RT). \tag{4}$$

Here, we introduce imperfections in the polarisation overlap of the photons from the two QDs, quantified by the classical interference visibility $(1-\epsilon)$. $\mathcal{V}$ represents the true two-photon overlap of the $|1_i, 1_j\rangle$ state.

Due to the finite $g^{(2)}(0)$ in the QD emission, the input states on the beamsplitter contain small multi-photon components with probabilities $P_n^{\mathrm{QD_m}}$,

$$|\psi_{\mathrm{in}}^{\mathrm{QD_m}}\rangle = P_0^{\mathrm{QD_m}}\,|0\rangle + P_1^{\mathrm{QD_m}}\,|1\rangle + P_2^{\mathrm{QD_m}}\,|2\rangle + \ldots \tag{5}$$

where $m = i, j$ denotes the emitters at the two input ports and $n = 0, 1, 2...$ represents the number of photons created by the $\pi$-pulse excitation. As the excitation pulse width is very short compared to the QD lifetime, the probability of creating the two-photon component by the $\pi$-pulse is much smaller than that of creating a single-photon state[6], i.e. $P_2^{\mathrm{QD_m}} \ll P_1^{\mathrm{QD_m}}$. We can relate $P_1^{\mathrm{QD_m}}$ and $P_2^{\mathrm{QD_m}}$ to the second-order correlation function $g^{(2)}(0)$ via:

$$g^{(2)}_{\mathrm{QD_m}} \simeq \frac{2 \cdot P_2^{\mathrm{QD_m}}}{\left(P_1^{\mathrm{QD_m}}\right)^2}. \tag{6}$$

Using this relation, the HOM probabilities for the $|1_i, 1_j\rangle$ and $|0_i, 2_j\rangle\,, |2_i, 0_j\rangle$ input states are expressed as:

$$\mathrm{HOM}_{11} = P_1^{\mathrm{QD_i}} P_1^{\mathrm{QD_j}} (T - R)^2 \tag{7}$$

$$\mathrm{HOM}_{20,02} = \frac{1}{2}\left[g^{(2)}_{\mathrm{QD_i}}\left(P_1^{\mathrm{QD_i}}\right)^2 + g^{(2)}_{\mathrm{QD_j}}\left(P_1^{\mathrm{QD_j}}\right)^2\right](2RT)\,. \tag{8}$$

Substituting Eq. 4 into $\mathrm{HOM}_{11}$ and assuming a slight imbalance in the two input photon-fluxes, i.e. $P_1^{\mathrm{QD_i}} \approx P_1^{\mathrm{QD_j}} + \eta$, the overall $\mathcal{V}_{\mathrm{Q}}$ probability is given by $\mathcal{V}_{\mathrm{Q}} = \mathrm{HOM}_{11} + \mathrm{HOM}_{20,02}$ with:

$$\mathrm{HOM}_{11} = P_1^{\mathrm{QD_i}}(P_1^{\mathrm{QD_i}} + \eta)\left[1 - 2RT - 2RT(1-\epsilon)^2\mathcal{V}\right], \tag{9}$$

$$\mathrm{HOM}_{20,02} = P_1^{\mathrm{QD_i}} \cdot \frac{1}{2}\left[(g^{(2)}_{\mathrm{QD_i}} + g^{(2)}_{\mathrm{QD_j}})(P_1^{\mathrm{QD_i}} + \eta) + (g^{(2)}_{\mathrm{QD_i}} - g^{(2)}_{\mathrm{QD_j}})\eta\right](2RT). \tag{10}$$

The last term in $\mathrm{HOM}_{20,02}$ vanishes since the difference in $g^{(2)}_{\mathrm{QD_i}}$ and $g^{(2)}_{\mathrm{QD_j}}$ is typically small, i.e. $(g^{(2)}_{\mathrm{QD_i}} - g^{(2)}_{\mathrm{QD_j}})\eta \sim 0$. Setting $\mathcal{V} = 0$ in the $\mathcal{V}_{\mathrm{Q}}$ expression, we arrive at the overall $\mathcal{V}_{\mathrm{C}}$ probability – if taking the small 2-photon component into consideration. Hence, we can extract the corrected visibility $\mathcal{V}$ from the raw visibility using $\mathcal{V}_{\mathrm{raw}} = \left(\mathcal{V}_{\mathrm{C}} - \mathcal{V}_{\mathrm{Q}}\right)/\mathcal{V}_{\mathrm{C}}$. The result reads:

$$\mathcal{V} = \frac{1}{(1-\epsilon)^2}\,\frac{R^2 + T^2}{2RT}\left[1 + \frac{1}{2}\Big(g^{(2)}_{\mathrm{QD_i}}(0) + g^{(2)}_{\mathrm{QD_j}}(0)\Big)\right]\,\mathcal{V}_{\mathrm{raw}}. \tag{11}$$

From Eq. 11, we extract the true indistinguishability of the two-QD photons: $\mathcal{V}^{\mathrm{QD1/2}} = (93.0 \pm 0.8)\%$ for the photons from QD1/QD2, and $\mathcal{V}^{\mathrm{QD1/3}} = (92.7 \pm 1.6)\%$ for the photons from QD1/QD3. Here, the reflection and transmission coefficients of the beamsplitter in two-QD HOM experiments are $R = 0.498$ and $T = 0.502$; the classical visibility $(1-\epsilon) = 0.996$. We re-calibrate the $g^{(2)}(0)$ values for the two-QD HOM setup, and use these values for correcting the two-QD HOM visibilities. We arrive at $g^{(2)}(0) = (2.05 \pm 0.27)\%$ for QD1, and $g^{(2)}(0) = (0.92 \pm 0.11)\%$ for QD2.

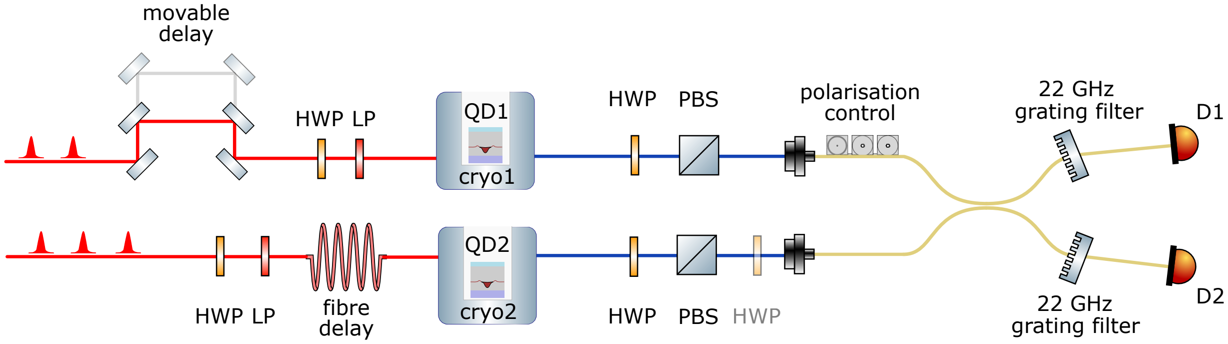


Supplementary Fig. 7. **Optical setup for Hong-Ou-Mandel experiments using two remote quantum dots.** The two GaAs QDs are located in two distant cryostats separated by 20-metre long fibres. Two separate excitation paths containing a movable delay on the QD1 side and an exchangeable fibre delay on the QD2 side are shown in red. The excitation pulses are synchronised. The excitation power can be separately adjusted (to the corresponding $\pi$-pulse power for each QD) using the combination of a HWP and a LP in each arm. Single photons from the two QDs (in blue) are sent to a fibre-based 50:50 beamsplitter. The HWP and the PBS on each of the collection paths set the polarisation of the QD photons to the co-polarised configuration. To distinguish the photons, we either insert another HWP to one of the collection paths (for the QD1-QD2 HOM measurement) or delay one photon temporally by half of the repetition period (by adding an additional fibre-delay in the excitation, e.g. for the QD1-QD3 HOM measurement). 22 GHz-bandwidth grating-based filters are inserted in both of the collection paths before the detectors.

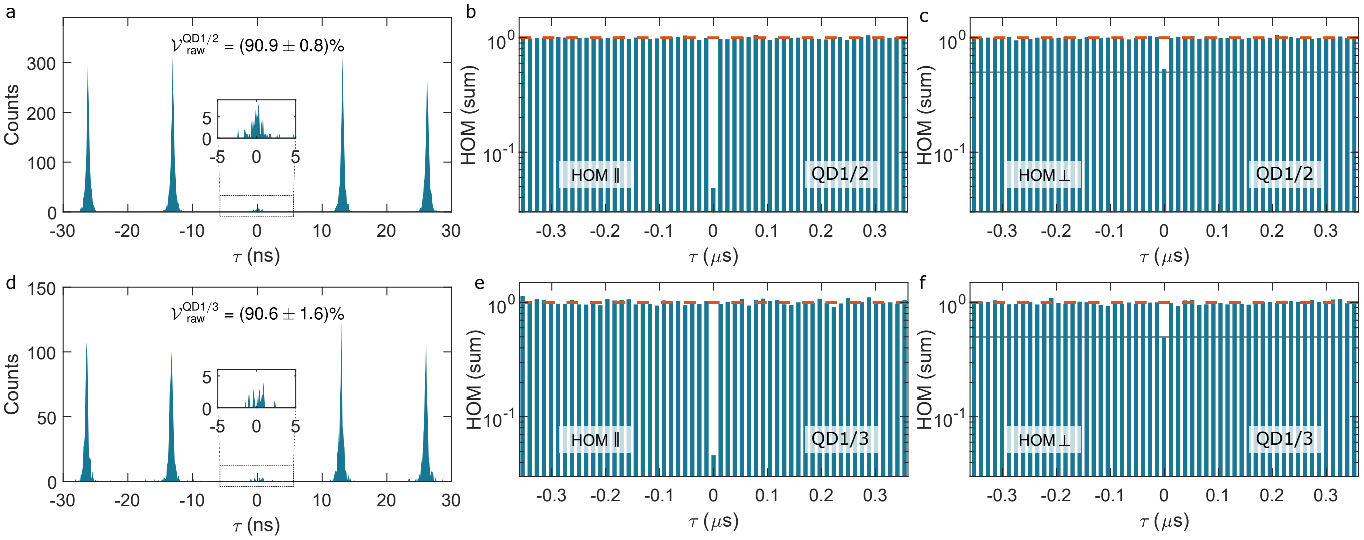


Supplementary Fig. 8. **Hong-Ou-Mandel interference between photons from remote quantum dots. (a-c)** Two-QD HOM experiments between photons from QD1 and QD2. The time-resolved two-QD HOM (in the co-polarised configuration) is plotted in (a), with the inset showing the zoom of the HOM central peak. Every peak in (a) is summed and normalised using a time bin of $T_{\text{bin}} = 13$ ns and shown as a bar chart in (b). In (c) we show a similar bar chart for the cross-polarised case. The grey line beneath the bars represents the expected 50% level for distinguishable photons. Comparing the heights of the central bars ($\tau = 0$) in (b) and (c), we extract the raw HOM visibility for QD1 and QD2, $\mathcal{V}_{\text{raw}}^{\text{QD1/2}} = (90.9 \pm 0.8)\%$. **(d-f)** Two-QD HOM experiments using photons from QD1 and QD3. Similar to (a-c), $\mathcal{V}_{\text{raw}}^{\text{QD1/3}} = (90.6 \pm 1.6)\%$ for QD1 and QD3.

## A. Theoretical modelling of the two-QD Hong-Ou-Mandel visibility

If two single-photons enter a symmetric beamsplitter from the two input arms $i$ and $j$, the probability that both input photons leave the beamsplitter through different output ports and become detected at times $t_0$ and $t_0 + \tau$ is given by[8]:

$$\mathcal{P}(t_0, \tau) = \frac{1}{4}|\zeta_i(t_0 + \tau)\zeta_j(t_0) - \zeta_j(t_0 + \tau)\zeta_i(t_0)|^2. \tag{12}$$

Here, $\zeta_{i,j}$ stands for the single-photon wave-functions from the two input arms. In our case, we describe the QD photons using a one-sided exponential decay,

$$\zeta_{i,j}(t) = \frac{1}{\sqrt{\tau_{i,j}}} H(t \pm \delta t/2) \cdot \exp\Big\{ -\frac{t \pm \delta t/2}{2\tau_{i,j}} - i[2\pi\nu_{i,j}t + \phi_{i,j}(t)]\Big\}, \tag{13}$$

with $\tau_{i,j}$ the radiative lifetime of the two QDs, $\nu_{i,j}$ the resonant frequency of the emitted photons. $\delta t$ is the difference in the two photons' arrival time at the beamsplitter. If the two photons from remote QDs arrive simultaneously, $\delta t = 0$. The Heaviside-function $H(t)$ makes sure that no photon exists prior to the excitation process. The time-dependent phase term $\phi_{i,j}(t)$ is included to model the fast dephasing process.

Since the HOM measurements take usually several hours, the time-resolved HOM interference, $\mathcal{G}^{(2)}(\tau)$, can be calculated by integrating $\mathcal{P}(t_0, \tau)$ over a long time period[8,9]:

$$\mathcal{G}^{(2)}(\tau) = \int_{-\infty}^{\infty} \langle\langle \mathcal{P}(t_0, \tau)\rangle\rangle \, \mathrm{d}t_0, \tag{14}$$

with $\langle\langle ... \rangle\rangle$ donating the statistical averaging.

$\mathcal{G}^{(2)}(\tau)$ is sensitive to both fast pure-dephasing and slow spectral fluctuations. Pure dephasing results in random fluctuations of the phase $\phi_{i,j}$. It is quantified by the dephasing rate $\Gamma^*_{i,j}$, leading to a modification in the overall dephasing rate $\gamma = \gamma_i + \gamma_j$ with $\gamma_{i,j} = 1/(2\tau_{i,j}) + \Gamma^*_{i,j}$ (here, $i$ and $j$ denote the two QDs). Spectral fluctuation can arise from noise (both spin noise and charge noise) in the semiconductor. It results in occasional frequency shifts in between the photon emission events, causing inhomogeneous broadening. The inhomogeneous broadening is often modelled with either a Gaussian[10,11] or a Lorentzian[12,13] distribution function. In the following, we discuss both the Gaussian- and Lorentzian-shaped spectral fluctuation and its influence on the two-photon interference.

• The noise results in a "Gaussian" spectral fluctuation:

In this case, the inhomogeneous broadening is described with a Gaussian probability distribution

$$p_{\mathrm{G}}(v) = \frac{1}{\sqrt{2\pi}\sigma} \exp[-\frac{1}{2}(\frac{\nu - \nu_0}{\sigma})^2], \tag{15}$$

where $\sigma_{i,j}$ donates the standard deviation of the spectral fluctuation for each QD (subscripts are omitted in Eq. 15). $\sigma_{i,j}$ is related to the full-width-at-half-maximum (FWHM) of the Gaussian fluctuation $\sigma'_{i,j}$ via $\sigma'_{i,j} = 2\sqrt{2\ln 2}\ \sigma_{i,j}$. For the overall effects on the two photons, we introduce the parameter $\Sigma$, where $\Sigma^2 = \sigma_i^2 + \sigma_j^2$. Following Ref. 9, we obtain the expression for $\mathcal{G}^{(2)}(\tau)$ :

$$\begin{aligned}\mathcal{G}^{(2)}(\tau) = \frac{1}{4(\tau_i + \tau_j)} \cdot \Bigg[ & H(\tau + \delta t) \cdot \exp\Big( -\frac{\tau + \delta t}{\tau_i}\Big) + H(-\tau - \delta t) \cdot \exp\Big(\frac{\tau + \delta t}{\tau_j}\Big) \\ & + H(\tau - \delta t) \cdot \exp\Big( -\frac{\tau - \delta t}{\tau_j}\Big) + H(-\tau + \delta t) \cdot \exp\Big(\frac{\tau - \delta t}{\tau_i}\Big) \\ & - 2 \cdot \exp\Big( -\frac{\delta t}{2T_-} - \frac{|\delta t|}{2T_+} - \gamma|\tau| - 2\pi^2\Sigma^2\tau^2\Big) \cdot \cos(2\pi\Delta\tau)\Bigg].\end{aligned} \tag{16}$$

Here, $1/T_\pm = 1/t_i \pm 1/t_j$, $\delta t$ represents the temporal delay of the two wave-packets and $\Delta = \nu_i - \nu_j$ their relative spectral detuning. $\mathcal{G}^{(2)}(\tau)$ describes the delay dependence of the central peak in the two-QD HOM experiment. The $\Gamma^*_{i,j}$ and $\Sigma$ terms in Eq. 16 represent the effects of fast dephasing and spectral fluctuations, respectively.

The overall probability of joint detection $\mathcal{P}$ at the two output ports is calculated by integrating $\mathcal{G}^{(2)}$ over $\tau$, $\mathcal{P} = \int_{-\infty}^{\infty} \mathcal{G}^{(2)}(\tau)\mathrm{d}\tau$. The results can be expressed as[9]:

$$\mathcal{P} = \frac{1}{2} \cdot \left( 1 - \frac{\mathrm{Re}[w(z)]}{\sqrt{2\pi}\Sigma(\tau_i + \tau_j)} \cdot e^{-|\delta t|/\tau_e} \right), \tag{17}$$

where $z = (2\pi\Delta + i\gamma)/(2\pi\sqrt{2}\Sigma)$, and $\tau_e$ stands for the lifetime of the "early" photon. $\mathrm{Re}[w(z)]$ is the real part of the Faddeeva function $w(z)$, which represents a Voigt profile[14]. The Voigt dependence (versus $\Delta$) is a result of the convolution between a Lorentzian function and a Gaussian function, which in turn comes from the Fourier transforms of the $\gamma$ (exponential) and $\Sigma$ (Gaussian) terms in Eq. 16. $\mathcal{P}$ is related to the two-QD HOM visibility via $\mathcal{V}_{\mathrm{calc}} = 1 - 2\mathcal{P}$. Here, for the value of $\mathcal{V}_{\mathrm{calc}}$, the effects of fast dephasing processes and spectral fluctuations are modelled, but experimental imperfections are not taken into account.

- The noise results in a "Lorentzian" spectral fluctuation:

$$p_{\rm L}(v) = \frac{1}{\pi}\frac{\xi/2}{(\nu-\nu_0)^2+(\xi/2)^2}, \tag{18}$$

with $\xi_{i,j}$ being the FWHM of the Lorentzian inhomogeneous broadening in the frequency domain for each QD. We introduce the parameter $\Xi$ accounting for the overall spectral fluctuations: $\Xi = \xi_i + \xi_j$. When assuming the spectral fluctuations of the two QDs are on the same level, $\xi_{i,j}$ becomes $\Delta\nu_S$ in the main text, i.e. $\xi_i = \xi_j = \Delta\nu_S$. The Lorentzian distribution function modifies the expression of $\mathcal{G}^{(2)}(\tau)$ to:

$$\begin{aligned}\mathcal{G}^{(2)}(\tau) = \frac{1}{4(\tau_i+\tau_j)}\cdot\Bigg[&H(\tau+\delta t)\cdot\exp\Big(-\frac{\tau+\delta t}{\tau_i}\Big) + H(-\tau-\delta t)\cdot\exp\Big(\frac{\tau+\delta t}{\tau_j}\Big)\\ &+H(\tau-\delta t)\cdot\exp\Big(-\frac{\tau-\delta t}{\tau_j}\Big) + H(-\tau+\delta t)\cdot\exp\Big(\frac{\tau-\delta t}{\tau_i}\Big)\\ &-2\cdot\exp\Big(-\frac{\delta t}{2T_-}-\frac{|\delta t|}{2T_+}-\gamma|\tau|-\Xi\pi|\tau|\Big)\cdot\cos(2\pi\Delta\tau)\Bigg].\end{aligned} \tag{19}$$

Here, instead of a Gaussian term we arrive at an exponential function $\exp(-\Xi\pi|\tau|)$ in the third line. This simplifies the expression for the joint detection probability $\mathcal{P}$ to:

$$\mathcal{P} = \frac{1}{2}\left(1-\frac{2(\gamma+\Xi\pi)}{(\gamma+\Xi\pi)^2+4\pi^2\Delta^2}\cdot\frac{e^{-|\delta t|/\tau_e}}{(\tau_i+\tau_j)}\right). \tag{20}$$

Now, $\mathcal{P}$ has a Lorentzian dependence on the detuning $\Delta$. It is related to the two-QD HOM visibility via $\mathcal{V}_{\rm calc} = 1-2\mathcal{P}$. For a perfect overlap of the two-photon wave-packets, i.e. $\tau_i = \tau_j = \tau_r$, $\delta t = 0$, $\Delta = 0$, the two-QD HOM visibility becomes:

$$\mathcal{V}_{\rm calc} = \frac{1}{1+(\Gamma^*_{\rm sum}+\pi\Xi)\cdot\tau_r}, \tag{21}$$

where $\Gamma^*_{\rm sum} = \Gamma^*_i + \Gamma^*_j$. In Eq. 21, $\Gamma^*_{\rm sum}$ and $\pi\Xi$ represent the half-width-at-half-maximum of the overall homogeneous and inhomogeneous broadening in angular frequency, respectively.

Neglecting the spectral fluctuation and assuming $\Gamma^*_j = \Gamma^*_i$, Eq. 21 simplifies to the well-known expression for the one-QD HOM visibility $\mathcal{V} = T_c/2\tau$, with $T_c$ defined as $1/\gamma_i$.

### B. Limitations on the two-QD Hong-Ou-Mandel visibilities

In an idealised situation, i.e. when there is no noise in both QD-environments, the effects of spectral fluctuations ($\Sigma = 0$ or $\Xi = 0$) and pure dephasing ($\Gamma^*_{i,j} = 0$) vanish. In this ideal case, we calculate the two-QD HOM visibility using Eq. 20 as a function of both the temporal delay $\delta t$ and spectral detuning $\Delta$ of the two wave-packets. The results are shown in Fig. 2 in the main text. In the calculations, the radiative decay rates of two QDs are taken from the exponential fits in Extended Data Fig. 2. When the two remotely created photons suffer no delay nor detuning, i.e. $\Delta = 0$ and $\delta t = 0$, we expect the visibility to be $\mathcal{V} = 99.95\%$ despite a slight difference (4.3%) in the decay rates of the two QDs. The dependence of the two-QD HOM visibility on the lifetime difference between the two QDs is depicted in Supplementary Fig. 9(a). The two-QD HOM visibility stays at a high level, e.g. close to 99% even when there is a 20% difference in the two-QD decay rates. Therefore, the difference in the decay rates is not the major limiting factor for the two-QD HOM experiment.

The measured visibility of the two-QD two-photon interference, $\mathcal{V} = (93.0 \pm 0.8)\%$, is around 7% less than the idealised expectation. We analyse this result in terms of the noise in the semiconductor and imperfections in the apparatus.

Assuming the visibility of the one-QD HOM experiment is primarily limited by the fast dephasing processes, we use it to determine the fast dephasing rates in the QD systems. The visibilities of the 13 ns one-QD HOM measurements are $\mathcal{V}^{\rm 13ns} = (97.8 \pm 1.8)\%$ for QD1 and $\mathcal{V}^{\rm 13ns} = (98.2 \pm 1.3)\%$ for QD2, respectively, i.e. both $\sim 2\%$ lower than the idealised expectation. In the calculation of the one-QD HOM visibility, we employ Eq. 21 assuming that the two photons have the same decay rate $\tau_i = \tau_j$ and perfect overlaps $\Delta = 0$, $\delta t = 0$. In the meantime, we ignore the influence of the slow spectral fluctuation process, $\Xi = 0$. We estimate how large the dephasing term needs to be

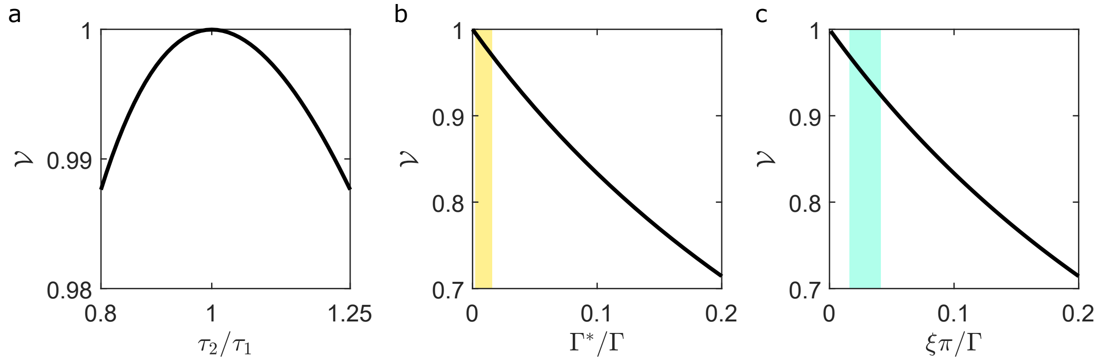


Supplementary Fig. 9. **Theoretical expectations of the two-quantum-dot Hong-Ou-Mandel visibility.** The two-QD HOM visibility is calculated using Eq. 20. All parameters are in the ideal limit ($\tau_1 = \tau_2$, $\Gamma_1^* = 0$, $\Gamma_2^* = 0$, $\sigma_1 = 0$, $\sigma_2 = 0$, $\delta t = 0$, $\Delta = 0$) except **(a)** the two QDs have different lifetimes ($\tau_1 \neq \tau_2$); **(b)** the two QDs suffer from pure dephasing processes parameterised by $\Gamma^*$ (normalised to the radiative decay rate $\Gamma$, $\Gamma^* = \Gamma_1^*/2 + \Gamma_2^*/2$); **(c)** environmental noise results in a Lorentzian-shaped spectral fluctuation (parameterised by the half-width-at-half-maximum of the inhomogeneous broadening $\xi\pi$ in angular frequency, and normalised by $\Gamma$, $\xi = \xi_1/2 + \xi_2/2$). The lifetime difference of the QDs plays only a minor role in the HOM visibility compared to the dephasing and spectral fluctuation processes. The coloured regions in (b) and (c) represent the estimated effects of the fast dephasing and slow spectral fluctuation in our QDs, respectively. The width of the coloured regions represents the error margin of the estimated $\Gamma^*$ and $\xi$.

in order to reach a visibility of 98%. From the calculations, this corresponds to $\Gamma^* = 34 \pm 25$ MHz for each QD (assuming $\Gamma^*_{\mathrm{QD1}} \sim \Gamma^*_{\mathrm{QD2}} = \Gamma^*$). The corresponding time is $1/\Gamma^* = 29 \pm 21$ ns: this is the time over which the exciton retains its phase in the absence of radiative decay. Here, the errors account for the uncertainty of the one-QD HOM visibility in the experiment. The dependence of the two-QD HOM visibility on the average dephasing rate $\Gamma^*$ is shown in Supplementary Fig. 9(b). The small dephasing rates of 34 MHz in both QD systems reduce the two-QD HOM visibility also to 98%.

Experimental imperfections such as the imbalance of the beamsplitter and the non-unity classical interference visibility have been accounted for in the estimation of the true two-QD HOM visibility $\mathcal{V}$. The remaining experimental imperfections are usually negligible for one-QD HOM experiments but might still influence the two-QD HOM. For example, two independent voltage sources are employed for frequency tuning the two QDs. These two voltage sources need to be stable over the measurement time-scale (in our case, around 2.5 hours) in order to maintain the two QDs in the same frequency. Although the mutual stability of the two voltage sources (LNHR DAC, Basel Precision Instruments) is high, we estimate a drift between the two voltage sources of $\sim \pm 20$ $\mu$V. Translating to frequency, this drift corresponds to an instability of 30 MHz (or $\sim 5\%$ of the QD linewidth), which leads to a reduction in HOM visibility of $\sim 0.3\%$ (i.e. from 98% to around 97.7%, estimated with the theoretical model). Besides, the dark counts from the SNSPDs also limit the measured visibility to a certain extent. We estimate a reduction of $\sim 0.5\%$ in the two-QD HOM visibility attributed to the dark counts. Nonetheless, experimental imperfections are thought to have a minor influence ($< 1\%$) on the measurements of $\mathcal{V}$.

The remaining difference between the experimental two-QD HOM visibility and the ideal value can be attributed to the slow noise in the semiconductor, the spectral fluctuations. The noise spectrum of some InGaAs QDs[12,13] is shown to have a Lorentzian spectral distribution. For the GaAs QDs, the preliminary data in Extended Data Fig. 3(b) suggests also a Lorentzian distribution. With Eq. 20, we calculate the two-QD HOM visibility as a function of the spectral fluctuation parameter $\Xi$, where $\Xi$ stands for the FWHM of the overall inhomogeneous broadening of both QDs in frequency, $\Xi = \xi_1 + \xi_2$. In the ideal case ($\Gamma^* = 0$, $\tau_1 = \tau_2$, $\delta t = 0$, $\Delta = 0$), the effect of spectral fluctuations is shown in Supplementary Fig. 9(c). In practice, the QDs also suffer from the impact of fast dephasing. Adding the dephasing rate $\Gamma^* = 34 \pm 25$ MHz, we estimate the spectral fluctuations in our systems to be $\Xi = 2 \times (34 \pm 15)$ MHz – this level of spectral fluctuation brings the calculated two-QD HOM visibility to the experimental result. In other words, the slow fluctuation of each QD results in on average a Lorentzian broadening of $\Delta\nu_S = 34 \pm 15$ MHz. This corresponds to a dephasing time $T_2^* = 1/(\pi\Delta\nu_S) = 9.1 \pm 3.9$ ns.

We compare the noise analysis based on the HOM visibilities with the measured spectral linewidths. For QD1 and QD2, the average spectral linewidth broadening is measured to be $55 \pm 26$ MHz; for QD1 and QD3, this value is $64 \pm 31$ MHz (from Lorentzian fits, see Extended Data Fig. 2). Subtracting the contribution of homogeneous broadening $\Delta\nu_H = \Gamma^*/\pi = 11 \pm 8$ MHz, we extract the inhomogeneous broadening $\Delta\nu_S^{\mathrm{exp}} = 43 \pm 27$ MHz for QD1 and QD2 pair, and $\Delta\nu_S^{\mathrm{exp}} = 53 \pm 32$ MHz for QD1 and QD3 pair. These results are compatible with the two-QD HOM analysis.

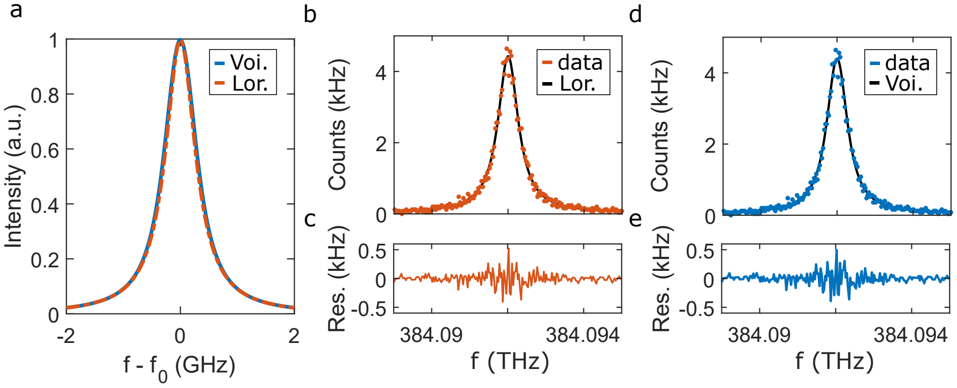


Supplementary Fig. 10. **A comparison of Voigt and Lorentzian lineshapes.** **(a)** Calculation of Voigt and Lorentzian lineshapes based on the experimental parameters. Red curve: Lorentzian profile calculated with a total broadening of $\Delta\nu_H + \Delta\nu_S = 45$ MHz plus the natural linewidth of $[1/(2\pi\tau_1) = 597$ MHz] (that is, in total, a FWHM of 642 MHz). Cyan curve: Voigt profile calculated with a Gaussian contribution (standard deviation $\sigma_{\text{avg}} = 95$ MHz) and a Lorentzian contribution [with FWHM of $\Delta\nu_H + 1/(2\pi\tau_1) = 608$ MHz]. The difference between the two lineshapes is hardly visible. **(b,c)** The Lorentzian fit to the QD1 spectrum and the residuals. The total Lorentzian broadening above the lifetime-limit is $50 \pm 17$ MHz. **(d,e)** The Voigt fit to the QD1 spectrum and the residuals. Here, we fixed the Lorentzian contribution to 608 MHz (FWHM). This yields a Gaussian contribution of $\sigma_{\text{fit}} = 70 \pm 43$ MHz. The Lorentzian function fits the data slightly better than the Voigt function.

We also present the analysis with a spectral fluctuation described by a Gaussian probability distribution. In this case, we rely on Eq. 17. Together with the dephasing rate $\Gamma^* = 34 \pm 25$ MHz, we estimate a spectral fluctuation of $\Sigma = \sqrt{2} \times (95 \pm 27)$ MHz – on average, the standard derivation of the spectral fluctuation is $\sigma_{\text{avg}} = 95 \pm 27$ MHz for each QD. The Gaussian contribution turns the QD spectrum into a Voigt profile. However, as $\sigma_{\text{avg}}$ is rather small compared to $1/(2\pi\tau_r)$ (the minimal Lorentzian width set by the radiative lifetime), the Voigt lineshape resembles the Lorentzian one [Supplementary Fig. 10(a)]. A comparison between the Lorentzian and Voigt fits to the QD1 spectrum are shown in Supplementary Fig. 10(b-e). The Gaussian width parameter ($\sigma_{\text{fit}} = 70 \pm 43$ MHz) extracted from the Voigt fit can be compatible with the $\sigma_{\text{avg}}$ determined from the two-QD HOM visibility. However, the Lorentzian function fits the data slightly better than the Gaussian function.

## C. Effects of Purcell enhancement

Thanks to the low noise behaviour in our GaAs QDs system, the visibility of one-QD and two-QD HOMs are close to perfect even without any Purcell enhancement.

Eq. 21 allows an estimation of the effect of Purcell enhancement on the one-QD and two-QD HOM visibility to be made. The Purcell effect reduces the radiative lifetime of the QD, $\tau_r$, by the Purcell factor $F_{\text{P}}$. This leads to an additional increase in one-QD and two-QD HOM visibilities. For single-QD photons, with only moderate Purcell enhancement, e.g. $F_{\text{P}} = 5$, the lifetime is shorten to $\tau_r \sim 50$ ps and the indistinguishability can be boosted above 99.5%. For the photons from remote QDs, a Purcell enhancement of $F_{\text{P}} = 10$ in each system is enough to increase the two-QD HOM visibility to above 99% provided that the present noise-level is preserved (assuming a Lorentzian noise spectrum, e.g. Extended Data Fig. 3; for a Gaussian noise spectrum the two-QD HOM visibility exceeds 99% for $F_{\text{P}} \sim 6$). Such a moderate Purcell enhancement has been realised in various nano-engineered platforms, such as integrated photonic-crystal cavities[15], micropillars[16], and open microcavities[17,18].

## D. Summary of previous studies

In Table I below, we summarise some previous experiments together with our results. Here, we focus on the experiments working with pulsed excitation scheme. Compared to CW excitation scheme[19–21], pulsed excitation allows the QD to be prepared in an excited state with high fidelity, which consequently leads to near-deterministic photon creation. Except for the work listed in the table, we note that the following work also reports two-photon interference between two separate QDs: Ref. [22–28]. The reported visibility in these work lies between 18% and 42%.

Here, He and co-workers demonstrated a high two-QD HOM visibility[29] with the help of both a narrow spectral filter and temporal post-selection (we estimate in this case the filtering and post-selection remove a significant part

of QD photons). The work by Reindl *et al.* holds the current published record of two-QD HOM visibility between GaAs QDs[30], $\mathcal{V}_{\mathrm{corr}} = 51 \pm 5\%$. Weber *et al.* successfully converted the frequency of two InGaAs QDs to telecom wavelengths and show two-photon interference visibility[31] of $29 \pm 3\%$. You *et al.* continue in this direction and have demonstrated two-QD HOM interference with a visibility[32] of $\mathcal{V}_{\mathrm{corr}} = 73 \pm 2\%$ with the help of Purcell enhancement. At almost the same time, we show the photons from separate QDs are mutually indistinguishable – $\mathcal{V}_{\mathrm{corr}} = 93\%$.

TABLE I. **An overview of two-photon interference experiments between photons from separate quantum dots**

| | He *et al.* [29] | Reindl *et al.* [30] | Weber *et al.* [31] | You *et al.* [32] | this work |
|---|---|---|---|---|---|
| Platform | InGaAs QDs | GaAs QDs | InGaAs QDs, frequency conversion | InGaAs QDs, frequency conversion | GaAs QDs |
| Excitation scheme, (upper-state occupation) | Pulsed excitation, Raman scheme | Pulsed phonon-assisted two-photon excitation (∼88% population) | Pulsed resonant excitation (near-unity population) | Pulsed resonant excitation (near-unity population) | Pulsed resonant excitation (near-unity population) |
| Spectral filtering, (filter bandwidth) | Narrow, $\Delta v_{\mathrm{fil}} \sim 0.5\Delta v_{\mathrm{QD}}$ | None | Broad, defined by the cavity | Broad, defined by the cavity | Broad, $\Delta v_{\mathrm{fil}} \sim 34\Delta v_{\mathrm{QD}}$ |
| Temporal post-selection | Narrow (3 ns window) | None | None | None | None |
| Photonic engineering | not given | None | Micropillar cavity | Micropillar and bullseye cavities | None |
| Filtering efficiency[a] | $< 50\%$[b] | Near-unity | Near-unity | Near-unity | Near-unity |
| Two-QD HOM visibility[c] | $V_{\mathrm{raw}}= (77{\pm}2)\%$ | $V_{\mathrm{raw}}= (45{\pm}3)\%$ $V_{\mathrm{corr}}= (51{\pm}5)\%$ | $V_{\mathrm{raw}} = (29{\pm}3)\%$ | $V_{\mathrm{raw}} = (67{\pm}2)\%$ $V_{\mathrm{corr}} = (73{\pm}2)\%$ | $V_{\mathrm{raw}} = (91{\pm}1)\%$ $V_{\mathrm{corr}} = (93{\pm}1)\%$ |

[a] Here we define the filtering efficiency as the ratio between the photon-counts after spectral or temporal filtering compared to the photon counts before filtering. We only consider the coherent part of the QD emission, i.e. photons in the zero-phonon line.
[b] Based on our estimation considering both the narrow spectral filter and temporal post-selection
[c] For Ref. [32] we do not include the consideration of narrow temporal post-selections

### Supplementary Note 3. The Optical Controlled-NOT Circuit with Remote-Quantum-Dot Photons

We have performed a proof-of-principle demonstration of an optical controlled-not (CNOT) circuit utilising the coherent photons from QD1 and QD2. The CNOT gate is equivalent to a controlled phase gate up to single-qubit operations. In this work, the CNOT functionality is realised based on two-photon interference in linear optics[1,33–35]. The optical setup consists of a combination of three partially polarising beamsplitters (PPBSs) working as a controlled phase gate and two half-wave plates (HWPs) as two Hadamard gates [Supplementary Fig. 11(a)].

The controlled phase (CZ) gate performs a $\pi$-phase shift conditioned by the two-qubit state $|11\rangle$, i.e.

$$a\,|00\rangle + b\,|01\rangle + c\,|10\rangle + d\,|11\rangle \xrightarrow{\mathrm{CZ}} a\,|00\rangle + b\,|01\rangle + c\,|10\rangle - d\,|11\rangle\,.$$

In the experiment, we define $|H\rangle = |0\rangle$, $|V\rangle = |1\rangle$. The $\pi$-phase shift is implemented via quantum interference at the central PPBS ($\mathrm{PPBS}_0$). The central PPBS exhibits perfect transmission for horizontal polarisation and 1/3 transmission for vertical polarisation. For the $|VV\rangle$ inputs from the two ports $i$ and $j$, if the two photons are indistinguishable, the central PPBS results in a total amplitude of $-1/3$ for the $|VV\rangle$:

$$t_V^i \cdot t_V^j + (ir_V^i \cdot ir_V^j) = \sqrt{\frac{1}{3}}\sqrt{\frac{1}{3}} - \sqrt{\frac{2}{3}}\sqrt{\frac{2}{3}} = -\frac{1}{3}. \tag{22}$$

Here, $t^{i,j}$ and $r^{i,j}$ are the amplitude transmission and reflection coefficients of the central PPBS, respectively. For the other three input states, i.e. $|HH\rangle$, $|HV\rangle$ and $|VH\rangle$, the central PPBS does not introduce any quantum interference. The amplitudes in the coincidence measurements are attenuated to 1/3 by the PPBSs on the two output arms

[see Supplementary Fig. 11(a); $\mathrm{PPBS}_1$ and $\mathrm{PPBS}_2$ each reduce the transmission of $H$-polarised light to 1/3]. For example, the $|HH\rangle$ output reads $\left(t_H^i t_H^j\right) \cdot \left(t_H^1 t_H^2\right) = \frac{1}{3}$, where $t_H^{1,2} = \sqrt{\frac{1}{3}}$ is the transmission amplitude of $\mathrm{PPBS}_1$ and $\mathrm{PPBS}_2$. Therefore, a CZ operation can be realised with an amplitude of 1/3 using the arrangement of three PPBSs in Supplementary Fig. 11(a), i.e. a success probability of 1/9.

### A. Alignment of the controlled-NOT setup

In reality, the PPBSs (Asahi Spectra) do not have perfect performance, e.g. the transmission (reflection) is not precisely 1/3 (2/3). The performance of PPBSs depends on the incident angle. To achieve optimal performance, we align the CNOT setup with the aim to fulfil the following three criteria[33,36]:

1. the reflectivity of $\mathrm{PPBS}_0$ for $H$-polarisation should be zero,
$$r_H^i = 0 = r_H^j; \tag{23}$$
2. the product of the reflection amplitudes of $\mathrm{PPBS}_0$ should be twice its transmission amplitudes,
$$\frac{r_V^i \cdot r_V^j}{t_V^i \cdot t_V^j} = 2; \tag{24}$$
3. the attenuation of $\mathrm{PPBS}_1$ and $\mathrm{PPBS}_2$ should balance the amplitudes of $H$- and $V$-polarised light,
$$t_H^i \cdot t_H^1 = t_V^i \cdot t_V^1, \tag{25}$$
$$t_H^j \cdot t_H^2 = t_V^j \cdot t_V^2. \tag{26}$$

In the experiment, these three conditions are mostly met:

1. $r_H^i = 0.0008,\ r_H^j = 0.0031;$
2. $t_V^i = \sqrt{0.3306},\ t_V^j = \sqrt{0.3355},\ r_V^i = \sqrt{0.6389},\ r_V^j = \sqrt{0.6645}$, such that
$$\frac{r_V^i \cdot r_V^j}{t_V^i \cdot t_V^j} = 1.96;$$
3. $t_H^1 = \sqrt{0.3237}, t_V^1 = \sqrt{0.9548}, t_H^2 = \sqrt{0.3236}, t_V^2 = \sqrt{0.9904}$, such that,
$$t_H^i \cdot t_H^1 = 1.0039 \cdot t_V^i \cdot t_V^1,$$
$$t_H^j \cdot t_H^2 = 0.9839 \cdot t_V^j \cdot t_V^2.$$

### B. Operation of the controlled-NOT gate

We test the gate performance in both the computational basis $|H\rangle / |V\rangle$ and the $|+\rangle / |-\rangle$ basis, where $|\pm\rangle = 1/\sqrt{2}(|H\rangle \pm |V\rangle)$. The input states are prepared using two half-wave plates [see Fig. 3(a) in the main text]. For every input state, the output states are measured simultaneously with four coincidence measurements. The coincidence events of each central peak in the four measurements are summed using $T_{\mathrm{bin}} = 13$ ns. The sum represents the count rates for each input-output relation. The coincidence count rates are converted to probabilities by normalising them with the overall coincidence counts of all four coincidence measurements. The probabilities are plotted in Fig. 3(b,c) and the numbers are shown in Supplementary Fig. 11(b,c) for the two measurement bases.

The fidelity of the CNOT gate, defined as the averaged probability of obtaining the expected output states, is calculated as[37,38],

$$\mathcal{F}_{ZZ} = \frac{1}{4}\Big[P(HH|HH) + P(HV|HV) + P(VH|VV) + P(VV|VH)\Big],$$
$$\mathcal{F}_{XX} = \frac{1}{4}\Big[P(++\,|++) + P(+-\,|--) + P(-+\,|-+) + P(--\,|+-)\Big].$$

a

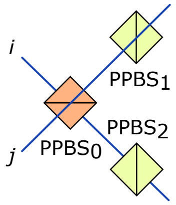


b

CNOT in the |H⟩/|V⟩ basis

| Out\In | HH | HV | VH | VV |
|---|---|---|---|---|
| HH | 0.938 | 0.008 | 0.004 | 0.006 |
| HV | 0.030 | 0.932 | 0.008 | 0.023 |
| VH | 0.026 | 0.008 | 0.139 | 0.837 |
| VV | 0.006 | 0.052 | 0.849 | 0.134 |

c

CNOT in the |+⟩/|−⟩ basis

| Out\In | ++ | +− | −+ | −− |
|---|---|---|---|---|
| ++ | 0.950 | 0.009 | 0.022 | 0.006 |
| +− | 0.030 | 0.135 | 0.004 | 0.852 |
| −+ | 0.012 | 0.011 | 0.928 | 0.004 |
| −− | 0.009 | 0.845 | 0.046 | 0.138 |

Supplementary Fig. 11. **A Sketch of the controlled-phase gate and truth tables for the controlled-not gate measured in two complementary bases.** **(a)** The central partially polarising beamsplitter ($\mathrm{PPBS}_0$) transmits $H$-polarised light while reflects partially $V$-polarised light. The other two PPBSs are flipped by 90° so that all $V$-polarised components are transmitted and $H$-polarised components are attenuated by 2/3. **(b,c)** Truth tables of the CNOT process in the $|H\rangle / |V\rangle$, and $|+\rangle / |-\rangle$ bases. The same results are visualised in Fig. 3(b,c) of the main text.

Here $P(\mathrm{I}_1\mathrm{I}_2|\mathrm{O}_1\mathrm{O}_2)$ represents the input-output probabilities of the CNOT operation. Substituting the probabilities from experimental results [Supplementary Fig. 11(b, c)] into the equations, we obtain $\mathcal{F}_{ZZ} = (88.90 \pm 5.34)\%$, and $\mathcal{F}_{XX} = (89.34 \pm 5.29)\%$.

We take the measurements in the $|H\rangle / |V\rangle$ basis as an example and analyse the limiting factors for each input state. For $|HH\rangle$ input, the signal in the $|HV\rangle$ and $|VV\rangle$ outputs arises probably because of imperfections in the PPBSs as well as the imprecision of the half-wave plate rotation; for the $|VH\rangle$ output, the non-zero values of $g^{(2)}(0)$ play a major role, together with the PPBS and HWP imperfections. The undesired outputs for the $|HV\rangle$ input state have similar origins. For $|VH\rangle$ and $|VV\rangle$ inputs, quantum interference between remote-QD photons plays a major role in the flip of the target qubit. Take the $|VV\rangle$ input as an example: measuring the $|VV\rangle$ output probability is in principle the same as a two-QD HOM experiment in which the count-rates of both QDs are reduced to 1/3. The unflipped $|VV\rangle$ output arises mostly from the $\sim 7\%$ imperfection in the two-QD HOM visibility ($\mathcal{V}_{\mathrm{corr}}^{\mathrm{QD1/2}} = 93.0\%$). The finite $|HH\rangle$ and $|HV\rangle$ outputs arise again due to the setup imperfections. To pin down the influence of the two-QD HOM visibility, we assume a perfect CNOT setup and set the values of $g^{(2)}(0)$ to be zero. In this case, we expect the CNOT process fidelity e.g. in the computational basis to be $\mathcal{F}_{ZZ} \sim 93.9\%$.

[1] He, Y.-M. *et al.* On-demand semiconductor single-photon source with near-unity indistinguishability. *Nat. Nanotechnol.* **8**, 213–217 (2013).
[2] Löbl, M. C. *et al.* Radiative Auger process in the single-photon limit. *Nat. Nanotechnol.* **15**, 558–562 (2020).
[3] Morrison, C. L. *et al.* A bright source of telecom single photons based on quantum frequency conversion. *Appl. Phys. Lett.* **118**, 174003 (2021).
[4] Kiršanskė, G. *et al.* Indistinguishable and efficient single photons from a quantum dot in a planar nanobeam waveguide. *Phys. Rev. B* **96**, 165306 (2017).
[5] Zhai, L. *et al.* Large-range frequency tuning of a narrow-linewidth quantum emitter. *Appl. Phys. Lett.* **117**, 083106 (2020).
[6] Fischer, K. A. *et al.* Signatures of two-photon pulses from a quantum two-level system. *Nat. Phys.* **13**, 649–654 (2017).
[7] Kuhlmann, A. V. *et al.* A dark-field microscope for background-free detection of resonance fluorescence from single semiconductor quantum dots operating in a set-and-forget mode. *Rev. Sci. Instrum.* **84**, 073905 (2013).
[8] Legero, T., Wilk, T., Kuhn, A. & Rempe, G. Time-resolved two-photon quantum interference. *Appl. Phys. B* **77**, 797 (2003).
[9] Kambs, B. & Becher, C. Limitations on the indistinguishability of photons from remote solid state sources. *New J. Phys.* **20**, 115003 (2018).
[10] Wang, H. *et al.* Near-Transform-limited single photons from an efficient solid-state quantum emitter. *Phys. Rev. Lett.* **116**, 213601 (2016).
[11] Sun, Z., Delteil, A., Faelt, S. & Imamoğlu, A. Measurement of spin coherence using Raman scattering. *Phys. Rev. B* **93**, 241302 (2016).
[12] Kuhlmann, A. V. *et al.* Charge noise and spin noise in a semiconductor quantum device. *Nat. Phys.* **9**, 570–575 (2013).
[13] Kuhlmann, A. V. *et al.* Transform-limited single photons from a single quantum dot. *Nat. Commun.* **6**, 8204 (2014).
[14] Abrarov, S. & Quine, B. Efficient algorithmic implementation of the Voigt/complex error function based on exponential series approximation. *Appl. Math. Comput.* **218**, 1894–1902 (2011).
[15] Liu, F. *et al.* High Purcell factor generation of indistinguishable on-chip single photons. *Nat. Nanotechnol.* **13**, 835 (2018).
[16] Wei, Y. *et al.* Tailoring solid-state single-photon sources with stimulated emissions. arXiv:2109.09284 (2021).
[17] Tomm, N. *et al.* A bright and fast source of coherent single photons. *Nat. Nanotechnol.* **16**, 399–403 (2021).
[18] Senellart, P., Solomon, G. & White, A. High-performance semiconductor quantum-dot single-photon sources. *Nat. Nanotechnol.* **12**, 1026–1039 (2017).
[19] Patel, R. B. *et al.* Two-photon interference of the emission from electrically tunable remote quantum dots. *Nat. Photonics* **4**, 632–635 (2010).
[20] Ates, S. *et al.* Two-photon interference using background-free quantum frequency conversion of single photons emitted by an InAs quantum dot. *Phys. Rev. Lett.* **109**, 147405 (2012).
[21] Konthasinghe, K. *et al.* Field-field and photon-photon correlations of light scattered by two remote two-level InAs quantum dots on the same substrate. *Phys. Rev. Lett.* **109**, 267402 (2012).
[22] Flagg, E. B. *et al.* Resonantly driven coherent oscillations in a solid-state quantum emitter. *Nat. Phys.* **5**, 203 (2009).
[23] Gold, P. *et al.* Two-photon interference from remote quantum dots with inhomogeneously broadened linewidths. *Phys. Rev. B* **89**, 035313 (2014).
[24] Giesz, V. *et al.* Cavity-enhanced two-photon interference using remote quantum dot sources. *Phys. Rev. B* **92**, 161302 (2015).
[25] Jöns, K. D. *et al.* Two-photon interference from two blinking quantum emitters. *Phys. Rev. B* **96**, 075430 (2017).
[26] Thoma, A. *et al.* Two-photon interference from remote deterministic quantum dot microlenses. *Appl. Phys. Lett.* **110**, 011104 (2017).
[27] Weber, J. H. *et al.* Overcoming correlation fluctuations in two-photon interference experiments with differently bright and independently blinking remote quantum emitters. *Phys. Rev. B* **97**, 195414 (2018).
[28] Zopf, M. *et al.* Frequency feedback for two-photon interference from separate quantum dots. *Phys. Rev. B* **98**, 161302 (2018).
[29] He, Y. *et al.* Indistinguishable tunable single photons emitted by spin-flip raman transitions in InGaAs quantum dots. *Phys. Rev. Lett.* **111**, 237403 (2013).
[30] Reindl, M. *et al.* Phonon-Assisted Two-Photon Interference from Remote Quantum Emitters. *Nano Lett.* **17**, 4090–4095 (2017).
[31] Weber, J. H. *et al.* Two-photon interference in the telecom C-band after frequency conversion of photons from remote quantum emitters. *Nat. Nanotechnol.* **14**, 23–26 (2018).
[32] You, X. *et al.* Quantum interference between independent solid-state single-photon sources separated by 300 km fiber. arXiv:2106.15545 (2021).
[33] Kiesel, N., Schmid, C., Weber, U., Ursin, R. & Weinfurter, H. Linear optics controlled-phase gate made simple. *Phys. Rev. Lett.* **95**, 210505 (2005).
[34] Crespi, A. *et al.* Integrated photonic quantum gates for polarization qubits. *Nat. Commun.* **2**, 1 (2011).
[35] Langford, N. K. *et al.* Demonstration of a simple entangling optical gate and its use in Bell-state analysis. *Phys. Rev. Lett.* **95**, 210504 (2005).
[36] Kiesel, N. *Experiments on multiphoton entanglement.* Ph.D. thesis, Ludwig Maximilian University of Munich (2007).
[37] Li, J.-P. *et al.* Heralded nondestructive quantum entangling gate with single-photon sources. *Phys. Rev. Lett.* **126**, 140501

(2021).
[38] Hofmann, H. F. Complementary classical fidelities as an efficient criterion for the evaluation of experimentally realized quantum operations. *Phys. Rev. Lett.* **94**, 160504 (2005).
